# Supplementary material for: CertiFair: A Framework for Certified Global Fairness of Neural Networks
Source: arXiv:2205.09927 source file (2022-05-20)
Supplement: Supplementary file 1 [file Appendix_A.tex]

\section{Datasets}
\label{appendix:datasets}
In this section, we provide a detailed description of the fairness datasets used in Section \ref{sec:exp}. We preprocess all the datasets such that all numerical features are scaled to $[0,1]$ and the categorical features are one-hot encoded. The datasets are split into train and test sets that amount for $70 \%$ and $30 \%$ of the actual data, respectively.

\textbf{Adult:} The adult dataset is considered one of the most commonly used datasets for fairness-aware classification studies. The task is to predict whether the annual income of an individual exceeds \$50000 US dollars based on demographic characteristics. We consider the sensitive attribute for this dataset to be gender, with the privileged group being males.

\textbf{German:} The German credit dataset is used for credit assessment, i.e. decide if granting a credit to an individual is risky or not. It contains 1000 instances with no missing values. 

\textbf{Compas:} The Compas dataset is used to predict whether a criminal will be re-offending within two years. It contains 5278 preprocessed instances. We consider the sensitive attribute for this dataset to be race, with the privileged group being Caucasian.

\textbf{Law School:} The dataset contains records for law school admission of different universities in the United States. The goal is to predict whether a law student will pass the bar exam. The dataset contains 112630 preprocessed records. We consider the sensitive attribute for this dataset to be race, with the privileged group being White.

\begin{table}[!b]
    \caption{Number of data points classified positively. This metric is important when investigating fairness of classifiers. A naive classifier that classifies all points positively is 100 \% fair.}
    \centering
    \begin{tabular}{c|c}
    \toprule
         Dataset& Positivity rate (\%)  \\ \hline
         Adult & 24.17\\
         German & 66.33\\
         Compas & 52.95\\
         Law School & 26.34\\
    \bottomrule
    \end{tabular}
    \label{tab:datasets_stats}
\end{table}

Table \ref{tab:datasets_stats} summarizes the number of positive labels in each of the datasets. It is important to compare the percentage of satisfaction of a fairness property with this value, because a naive classifier can achieve 100 \% fairness by classifying all points positevly.
