# Supplementary material for: CertiFair: A Framework for Certified Global Fairness of Neural Networks
Source: arXiv:2205.09927 source file (2022-05-20)
Supplement: Supplementary file 2 [file Appendix_C.tex]

\section{Additional experiments}
\label{appendix:additional_exp}
We provide additional experiments similar to the ones in Table \ref{tab:exp3} for different values of the regularization parameter $\lambda_f$. Specifically, we consider properties of class $\mathcal{P}_2$ and compare between the impact of the global regularizer $\mathcal{L}_F^g$ and $\mathcal{L}_F^l$ for five randomly picked values of $\lambda_f \in \{0.01,0.03,0.07,0.1,0.5\}$. We observe that the global regularizer is able to enforce the fairness property with small values of $\lambda_f$, but after a certain threshold, the fairness loss dominates the loss and the accuracy starts to decrease. The local fairness regularizer seems to have very small effect for small values of $\lambda_f$ but starts to improve fairness for larger values starting from $\lambda_f=0.1$ for this set of properties and datasets. 

The data in Table~\ref{tab:app1} enforces our conclusions in Section 5.3 that the global fairness regularizer outperforms the local fairness regularizer in terms of providing better balance of fairness and accuracy. For example, in the German dataset, the local fairness regularizer was able to achieve 100\% fairness for $\lambda_f = 0.5$ but with a drop of accuracy from $75.30\%$ to $68.3\%$. On the other hand, the global fairness was able to achieve the same 100\% fairness with a much smaller $\lambda_f = 0.03$ and a reduction in the accuracy from $75.30\%$ to $73\%$. The same conclusion can be drawn among the Adult and Compas datasets.

% Please add the following required packages to your document preamble:
% \usepackage{graphicx}
\begin{table}[!h]
\centering
\caption{Comparison between global and local fairness regularizers for varying values of $\lambda_f$}
\label{tab:app1}
%\resizebox{\textwidth}{!}{%
\begin{tabular}{c|l|lll|lll}
\toprule
$\lambda_f$ & Dataset & \multicolumn{3}{c|}{Test Accuracy (\%)} & \multicolumn{3}{c}{Certified Fairness(\%)} \\
        & & Base & $\mathcal{L}_f^g$              & $\mathcal{L}_f^l$               & Base & $\mathcal{L}_f^g$              & $\mathcal{L}_f^l$                   \\ \hline
&Adult   & 84.55& 84.33           & 85.24           & 6.40 & 84.11                 & 29.21                \\
0.001& German  & 75.30& 73.00              & 74.33           & 8.64 & 95.06                 & 17.28                \\
&Compas  & 68.30 & 67.86           & 68.87           & 47.22 & 44.44                 & 16.66                \\
&Law     & 87.60 & 86.39           & 87.39           & 6.87 & 21.45                 & 6.04        \\ \bottomrule        
%\end{tabular}%
%}
% \end{table}
% % Accuracy: 84.55, 75.30, 68.30, 87.60
% % Fairness: 6.4062, 8.64, 47.22, 6.87
% \begin{table}[!h]
% \centering
% \caption{Comparison between global and local fairness regularizers with $\lambda_f=0.03$}
% \label{tab:app2}
%\resizebox{\textwidth}{!}{%
% \begin{tabular}{lllll}
% \toprule
%&Dataset & \multicolumn{2}{c}{Test Accuracy (\%)} & \multicolumn{2}{l}{Certified Fairness(\%)} \\
%        & $\mathcal{L}_f^g$              & $\mathcal{L}_f^l$               & $\mathcal{L}_f^g$              & $\mathcal{L}_f^l$                   \\ \hline
&Adult   & 84.55& 84.05	&84.76	& 6.40 & 95.83	&33.22              \\
0.003&German  & 75.30 & 73.00	&72.00	& 8.64 & 100.00	&13.58                \\
&Compas  & 68.30 & 67.42	&68.18	& 47.22 & 97.22	&19.44               \\
&Law     & 87.60 & 76.86	&86.64	& 6.87 & 76.87	&0.83        \\ \bottomrule        
% \end{tabular}%
% %}
% \end{table}
% \begin{table}[!h]
% \centering
% \caption{Comparison between global and local fairness regularizers with $\lambda_f=0.07$}
% \label{tab:app3}
% %\resizebox{\textwidth}{!}{%
% \begin{tabular}{lllll}
% \toprule
% Dataset & \multicolumn{2}{c}{Test Accuracy (\%)} & \multicolumn{2}{l}{Certified Fairness(\%)} \\
%         & $\mathcal{L}_f^g$              & $\mathcal{L}_f^l$               & $\mathcal{L}_f^g$              & $\mathcal{L}_f^l$                   \\ \hline
&Adult   & 84.55& 83.75	&84.88	& 6.40 &100.00	&41.40              \\
0.007&German  & 75.30 & 72.66	&71.33	& 8.64 &100.00	&22.22              \\
&Compas  & 68.30 & 64.89	&68.62	& 47.22 &100.00	&33.33              \\
&Law     & 87.60 & 74.21	&85.89	&6.87 &100.00	&1.66        \\ \bottomrule        
% \end{tabular}%
% %}
% \end{table}
% %
% %
% \begin{table}[!ht]
% \centering
% \caption{Comparison between global and local fairness regularizers with $\lambda_f=0.1$}
% \label{tab:app4}
% %\resizebox{\textwidth}{!}{%
% \begin{tabular}{lllll}
% \toprule
% Dataset & \multicolumn{2}{c}{Test Accuracy (\%)} & \multicolumn{2}{l}{Certified Fairness(\%)} \\
%         & $\mathcal{L}_f^g$              & $\mathcal{L}_f^l$               & $\mathcal{L}_f^g$              & $\mathcal{L}_f^l$                   \\ \hline
&Adult   & 84.55 & 83.43	&84.88	& 6.40 &100.00	&50.78              \\
0.1&German  & 75.30 & 72.66	&70.33	& 8.64 &100.00	&33.33            \\
&Compas  & 68.30 &65.21	&67.42	& 47.22 &100.00	&36.11              \\
&Law     & 87.60 & 73.92	&85.44	&6.87 &99.79	&1.45        \\ \bottomrule        
% \end{tabular}%
% %}
% \end{table}
% %
% %
% \begin{table}[!ht]
% \centering
% \caption{Comparison between global and local fairness regularizers with $\lambda_f=0.5$}
% \label{tab:app5}
% %\resizebox{\textwidth}{!}{%
% \begin{tabular}{lllll}
% \toprule
% Dataset & \multicolumn{2}{c}{Test Accuracy (\%)} & \multicolumn{2}{l}{Certified Fairness(\%)} \\
%         & $\mathcal{L}_f^g$              & $\mathcal{L}_f^l$               & $\mathcal{L}_f^g$              & $\mathcal{L}_f^l$                   \\ \hline
&Adult   & 84.55 & 82.56	&84.82	& 6.40 &100.00	&57.65            \\
0.5&German  & 75.30 & 69.30	&68.30	& 8.64 &100.00 	&100.00            \\
&Compas  & 68.30 &64.90	&65.40		& 47.22 &100.00	&66.66              \\
&Law     & 87.60 & 73.71	&81.01	&6.87 &100.00	&76.04        \\ \bottomrule        
\end{tabular}%
%}
\end{table}
