# Supplementary material for: CertiFair: A Framework for Certified Global Fairness of Neural Networks
Source: arXiv:2205.09927 source file (2022-05-20)
Supplement: Supplementary file 3 [file Appendix_B.tex]

\section{Fairness constraints}
\label{appendix:fair_constrnts}
In this section we provide a detailed explanation of the $\mathcal{P}_2$ fairness properties used to generate Table \ref{tab:exp3}

\textbf{Adult:} The numerical domain is defined as $D_\phi = [0.4,1] \times [0.5,0.7] \times [0,0.3], \times [0,0.2] \times [0.5,0.75]$. The similarity parameter $\delta_i = 0.05 \quad \forall i \in  \{1,\ldots n\}$

\textbf{German:} The numerical domain is defined as $D_\phi = [0,1]^n$. The similarity parameter $\delta_i = 0.05 \quad \forall i \in  \{1,\ldots n\}$.

\textbf{Compas:} The numerical domain is defined as $D_\phi = [0,1]^n$. The similarity parameter $\delta_i = 0.02 \quad \forall i \in  \{1,\ldots n\}$.

\textbf{Law School:} The numerical domain is defined as $D_\phi = [0,1]^n$. The similarity parameter $\delta_i = 0.03 \quad \forall i \in  \{1,\ldots n\}$.
